# Supplementary material for: $L_2$BN: Enhancing Batch Normalization by Equalizing the $L_2$ Norms of Features
Source: arXiv:2207.02625 source file (2023-03-21)
Supplement: Supplementary file 1 [file L2BN_SupplementaryMaterial_arxiv-V1.pdf]

# Supplementary Material

## A The Minimum Angle between Pairwise Class Centers for Figure 4

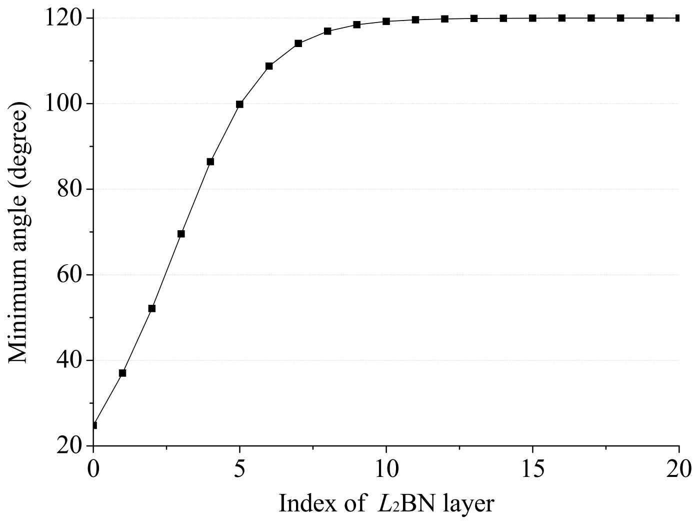


Figure 1: The minimum angle of each $L_2$BN layer in the case of Figure 4 of the paper.

In Figure 4 of the paper, we use an ellipsis to indicate the evolution of class centers affected by multiple layers of $L_2$BN, due to limited space. Here, to be more clear, we visualize the minimum angle of each $L_2$BN layer in Figure 1. We can see that the minimum angle continues to grow as the number of layers increases. After the tenth layer, the minimum angle basically stays at the maximum. Therefore, the proposed $L_2$BN can enlarge the discrepancy of inter-class features.

## B Training Settings for Image Classification Experiments

| Dataset | Model | LR | LR Scheduler | WD | BS | Epochs | Warm-up |
|---|---|---|---|---|---|---|---|
| CIFAR100 | ResNet | 0.1 | cosine, min_lr=0 | 5e-4 | 128 | 200 | None |
| | DenseNet | 0.1 | [150, 225], gamma=0.1 | 1e-4 | 64 | 300 | None |
| | VGG | 0.1 | cosine, min_lr=0 | 5e-4 | 128 | 200 | None |
| | RegNet | 1.0 | cosine, min_lr=0 | 5e-4 | 512 | 200 | 5 epochs |
| | ResNeXt | 0.1 | cosine, min_lr=0 | 5e-4 | 128 | 300 | None |
| ImageNet | ResNet | 0.2 | cosine, min_lr=0 | 5e-5 | 256 | 100 | None |
| | ResNeXt | 0.2 | cosine, min_lr=0 | 5e-5 | 256 | 100 | None |

Table 1: Experimental settings on CIFAR100 and ImageNet. LR denotes learning rate, WD denotes weight decay, and BS denotes batch size.

The optimizer is SGD [2] with a Nesterov momentum [3] of 0.9. The simple data augmentation in [1] is used in all the experiments of this part. Besides, the training of RegNet models uses $mixup$ [5] with $\alpha = 0.5$ and label smoothing [4] with a smoothing parameter of 0.1. Other hyper-parameters and settings are detailed in Table 1, which are basically the same as those in the original papers.

# C More $IIR$ Curves for the Image Classification Experiments

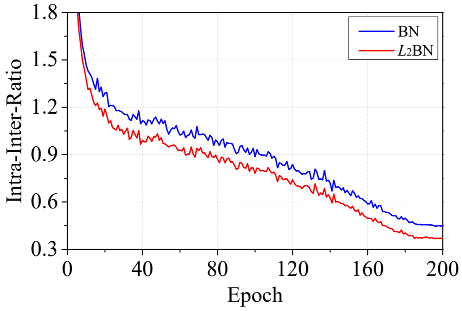


(a) *IIR* curves of RegNet-X

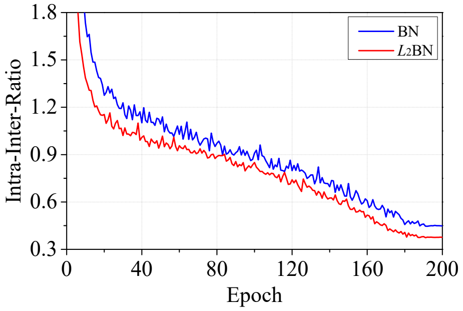


(b) *IIR* curves of RegNet-Y

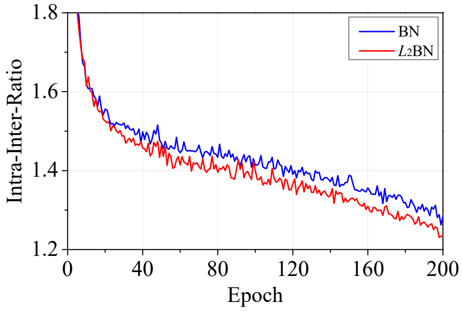


(c) *IIR* curves of ResNet-20

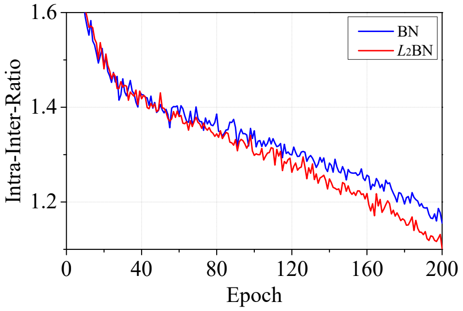


(d) *IIR* curves of ResNet-32

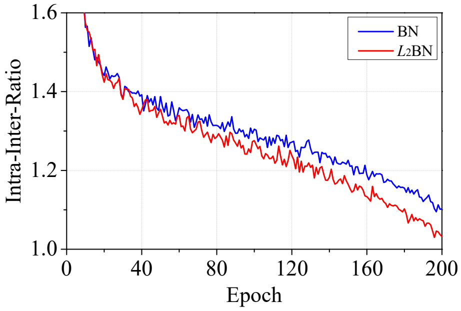


(e) *IIR* curves of ResNet-44

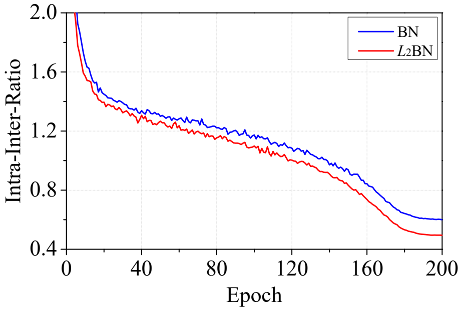


(f) *IIR* curves of ResNet-110

Figure 2: The comparison of $IIR$ curves on training data of CIFAR100. $L_2$BN achieves consistently smaller $IIR$ across the whole training.

Figure 2 shows more $IIR$ comparisons between BN and $L_2$BN. The $L_2$BN achieves consistently smaller $IIR$ across the whole training process, which enhances the advantages of $L_2$BN.

## References


[1] Chen-Yu Lee, Saining Xie, Patrick Gallagher, Zhengyou Zhang, and Zhuowen Tu. Deeply-supervised nets. In *Artificial Intelligence and Statistics*, pages 562–570, 2015.

[2] David E Rumelhart, Geoffrey E Hinton, and Ronald J Williams. Learning representations by back-propagating errors. *nature*, 323(6088):533–536, 1986.

[3] Ilya Sutskever, James Martens, George Dahl, and Geoffrey Hinton. On the importance of initialization and momentum in deep learning. In *International conference on machine learning*, pages 1139–1147. PMLR, 2013.

[4] Christian Szegedy, Vincent Vanhoucke, Sergey Ioffe, Jon Shlens, and Zbigniew Wojna. Rethinking the inception architecture for computer vision. In *Proceedings of the IEEE conference on computer vision and pattern recognition*, pages 2818–2826, 2016.

[5] Hongyi Zhang, Moustapha Cisse, Yann N Dauphin, and David Lopez-Paz. mixup: Beyond empirical risk minimization. *arXiv preprint arXiv:1710.09412*, 2017.
