# Supplementary material for: $L_2$BN: Enhancing Batch Normalization by Equalizing the $L_2$ Norms of Features
Source: arXiv:2207.02625 source file (2023-03-21)
Supplement: Supplementary file 2 [file SupplementaryMaterial.pdf]

# Supplementary Material

## A Training Settings for Image Classification Experiments

| Dataset  | Model    | LR  | LR Scheduler          | WD   | BS  | Epochs | Warm-up  |
|----------|----------|-----|-----------------------|------|-----|--------|----------|
| CIFAR100 | ResNet   | 0.1 | cosine, min_lr=0      | 5e-4 | 128 | 200    | None     |
|          | DenseNet | 0.1 | [150, 225], gamma=0.1 | 1e-4 | 64  | 300    | None     |
|          | VGG      | 0.1 | cosine, min_lr=0      | 5e-4 | 128 | 200    | None     |
|          | RegNet   | 0.5 | cosine, min_lr=0      | 5e-4 | 512 | 200    | 5 epochs |
| ImageNet | ResNet   | 0.2 | cosine, min_lr=0      | 5e-5 | 256 | 100    | None     |
|          | ResNeXt  | 0.2 | cosine, min_lr=0      | 5e-5 | 256 | 100    | None     |

Table 1: Experimental settings on CIFAR100 and ImageNet. LR denotes learning rate, WD denotes weight decay, and BS denotes batch size.

The optimizer is SGD [2] with a Nesterov momentum [3] of 0.9. The simple data augmentation in [1] is used in all the experiments of this part. Besides, the training of RegNet uses *mixup* [5] with  $\alpha = 0.5$  and label smoothing [4] with a smoothing parameter of 0.1. Other hyper-parameters and settings are detailed in Table 1, which are basically the same as those in the original papers.

## B More $IIR$ Curves for Image Classification Experiments

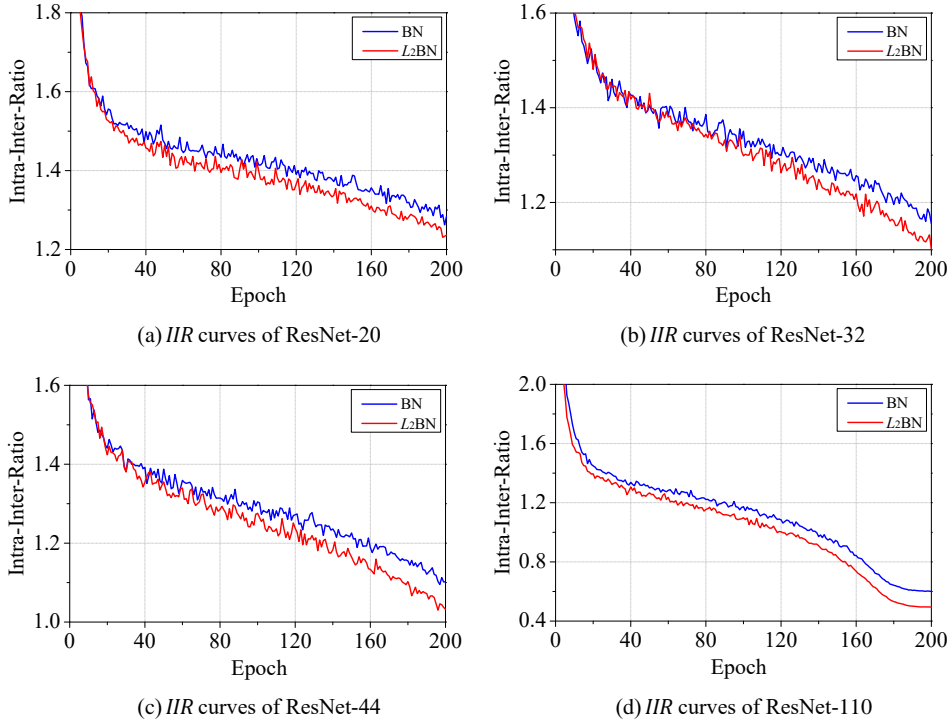

Figure 1: The comparison of  $IIR$  curves on training data of CIFAR100.  $L_2$ BN achieves consistently smaller  $IIR$  across the whole training.

Figure 1 shows more  $IIR$  comparisons between BN and  $L_2$ BN. The  $L_2$ BN achieves consistently smaller  $IIR$  across the whole training process, which enhances the advantages of  $L_2$ BN.

## References

- [1] Chen-Yu Lee, Saining Xie, Patrick Gallagher, Zhengyou Zhang, and Zhuowen Tu. Deeply-supervised nets. In *Artificial Intelligence and Statistics*, pages 562–570, 2015.
- [2] David E Rumelhart, Geoffrey E Hinton, and Ronald J Williams. Learning representations by back-propagating errors. *nature*, 323(6088):533–536, 1986.
- [3] Ilya Sutskever, James Martens, George Dahl, and Geoffrey Hinton. On the importance of initialization and momentum in deep learning. In *International conference on machine learning*, pages 1139–1147. PMLR, 2013.
- [4] Christian Szegedy, Vincent Vanhoucke, Sergey Ioffe, Jon Shlens, and Zbigniew Wojna. Rethinking the inception architecture for computer vision. In *Proceedings of the IEEE conference on computer vision and pattern recognition*, pages 2818–2826, 2016.
- [5] Hongyi Zhang, Moustapha Cisse, Yann N Dauphin, and David Lopez-Paz. mixup: Beyond empirical risk minimization. *arXiv preprint arXiv:1710.09412*, 2017.
